# Supplementary material for: The Forecast Trap
Source: arXiv:2207.10193 source file (2022-07-20)
Supplement: Supplementary file 1 [file appendix-A.pdf]

# Appendix A: Forecast Trap in a Multi-Species Model

Carl Boettiger

This appendix illustrates how the forecast trap can emerge in choosing between two alternative three-species models which may be used to manage a partially observed five-species system. The underlying dynamics for the simulated "true" system are based on the five-dimensional model of a herring fishery presented in Brias & Munch (2021). I have used the model parameters from Brias & Munch (2021), which were selected to ensure co-existence of the five species as outlined in their paper. Following Brias & Munch (2021), we assume three species of herring, $X_1$, $X_2$, $X_3$ are preyed upon by

$$x_{1,t+1} = s_{1,t} \exp\left(1.0213 - s_{1,t} - 0.0861 s_{2,t} - 0.3141 s_{3,t} - 0.7252 s_{4,t} - 0.2445 x_{5,t} + \epsilon_{1,t}\right) \quad (1)$$
$$x_{2,t+1} = s_{2,t} \exp\left(1.0289 - 0.4765 s_{1,t} - s_{2,t} - 0.1370 s_{3,t} - 0.9811 s_{4,t} - 0.0915 x_{5,t} + \epsilon_{2,t}\right) \quad (2)$$
$$x_{3,t+1} = s_{3,t} \exp\left(1.0207 - 0.3193 s_{1,t} - 0.3461 s_{2,t} - s_{3,t} - 0.6367 s_{4,t} - 0.8716 x_{5,t} + \epsilon_{3,t}\right) \quad (3)$$
$$x_{4,t+1} = s_{4,t} \exp\left(0.7252 s_{1,t} + 0.9811 s_{2,t} + 0.6367 s_{3,t} - s_{4,t} + \epsilon_{4,t}\right) \quad (4)$$
$$x_{5,t+1} = x_{5,t} \exp\left(0.2445 s_{1,t} + 0.0915 s2, t + 0.8716 s3, t - x_{5,t} + \epsilon_{5,t}\right) \quad (5)$$

where

$$s_{i,t} = x_{i_t}\left(1 - u_{i,t}\right)$$

$$\epsilon_{i,t} \overset{iid}{\sim} \mathcal{N}(0, \sigma_i)$$

We will assume this is the "true" model, which is unknown to managers.

Herring are harvested together, $u_1 = u_2 = u_3 = u_{\text{prey}}$, while bass are harvested at effort $u_{predator}$. The manager's utility in year $t$ is given by

$$R(\vec{x}_t, \vec{u}_t) = w_3 x_5 + w_2 x_4 + \sum_{i}^{1,2,3} w_1 x_i \quad (6)$$

We will consider the case which places 50% of the weight on the cormorant conservation objective, $w_3 = 0.5$, and 25% weight on the harvest of bass and herring respectively, $w_2 = w_1 = 0.25$.

In contrast to Brias & Munch (2021), we will assume that the manager must simply select the harvest efforts $u_{\text{prey}} \in [0, 1]$ and $u_{\text{predator}} \in [0, 1]$ to be used over the duration of the management scenario, rather than being able to adjust these annually. In most real-world systems it is not possible to measure all variables which influence the dynamics, some dimensions are treated as latent variables of the model. To illustrate this, we will assume that the manager observes only the population abundance of bass $x_{4,t}$, and cormorants, $x_{5,t}$, but not the population size of any of the three species of herring.

### Model A

Model A is a possible 3-species approximation that produces more accurate forecasts but leads to substantially worse management outcomes This model treats the three species of herring collectively as $x_1$. As with the original Brias & Munch (2021) model, parameters are not based directly on historical fisheries data, but have been selected to be consistent with simulations of the observed variables from the "true" model of Brias & Munch (2021), bass biomass $x_4$ and herring biomass $x_5$.

$$x_{1,t+1} = s_{1,t} \exp(3 - 8s_{1,t} - 0.9s_4 - 0.9 * x_{5,t} + \epsilon_{1,t}) \tag{7}$$
$$x_{4,t+1} = s_{4,t} \exp(0.1s_{1,t} - s_{4,t} + \epsilon_{4,t}) \tag{8}$$
$$x_{5,t+1} = x_{5,t} \exp(0.3s_{1,t} - x_5 + \epsilon_{5,t}) \tag{9}$$

### Model B

Model B is a structurally different model which postulates a further simplification of the dynamics. This slightly over-simplified approximation does not produce very accurate forecasts, but nevertheless leads to good management decisions.

$$x_{1,t+1} = s_{1,t} \exp(0.1 - 2.00s_{1,t} + \epsilon_{1,t}) \tag{10}$$
$$x_{4,t+1} = s_{4,t} \exp(1.45 - 2.75s_{1,t} + \epsilon_{4,t}) \tag{11}$$
$$x_{5,t+1} = 0.25x_{5,t} \tag{12}$$

Our alternate model has several oversimplifications: (1) it treat all three herring species as a single species, (2) it fails to capture the coupled predator-prey dynamics between bass and herring, (3) it oversimplifies the cormorant dynamics, assuming the cormorant population is determined to be a fixed fraction of the herring, and ignoring the impact of cormorant's predation on the herring itself. (4) Lastly, our model will overestimate the mortality introduced on herring by a given fishing effort. These elements are all obviously wrong, but not so arbitrary as to be inconceivable as a candidate model. Researchers frequently consider models which make oversimplifications all the time, and rely on model choice processes to weed them out.

The parameterization chosen for the oversimplified 3 species model can reasonably reproduce the un-fished dynamics. Under any harvesting regime or other influence that perturbs the system significantly far from the un-fished equilibrium co-existence state of the model quickly reveals the poor forecasting ability of this model. Nevertheless, solving for the optimal policy (under the same constraints of constant harvest fractions as we consider for the true model) results in a harvest policy which provides nearly optimal performance.

# Software implementation

```
library(tidyverse)
```

```
## helper funs
format_sim <- function(df) {
  df %>%
    transmute(time = time, cormorant = x5, bass = x4, herring = x1 + x2 + x3, r = r) %>%
    pivot_longer(any_of(c("cormorant", "bass", "herring")),
      names_to = "species",
```

```
      values_to = "biomass"
    )
}

clip <- function(x, lower = 0, upper = 1) {
  x[x <= lower] <- lower
  x[x >= upper] <- upper
  x
}
```

Define the reward for a given state,action pair and the net utility

```
## Compute the reward associated with a given simulation df given
## rates for prey and predator species (x[1],x[2])
reward <- function(df,
                   x,
                   w3 = 0.5, # Conservation value
                   w2 = 0.25, # Predator harvest value
                   w1 = 1 - (w2 + w3), # Prey harvest value
                   delta = 0.999) {
  u_prey <- clip(x[1], 0, 1)
  u_pred <- clip(x[2], 0, 1)
  R <-
    w1 * u_prey * (df$x1 + df$x2 + df$x3) +
    w2 * u_pred * df$x4 +
    w3 * df$x5
  t <- seq_along(R)
  as.numeric(R %*% delta^t)
}

# Function to be optimized for fixed choice of harvest rates x[1],x[2]
utility <- function(x, f, ...) {
  u_prey <- clip(x[1], 0, 1)
  u_pred <- clip(x[2], 0, 1)
  df <- f(u_prey, u_pred, ...)

  # average accross the reps
  df <- df %>%
    group_by(time) %>%
    summarise(across(.fns = mean))

  # negative since optimizer minimizes
  -reward(df, x)
}
```

# Model definitions

## True five species-model

```
# x1,x2,x3 Herring (Prey)
# x4 Bass (predator)
```

```r
# x5 Cormorant (conservation target, predator)
model_5sp <- function(u_prey = 0.5,
                      u_pred = 0.5,
                      sigma = 0.01,
                      x1o = 0.44, # unfished equib
                      x2o = 0.17,
                      x3o = 0.186,
                      x4o = 0.600,
                      x5o = 0.280,
                      Tmax = 50,
                      reps = 40) {
  df <- tibble()
  for (r in 1:reps) {
    x1 <- x2 <- x3 <- x4 <- x5 <- numeric(Tmax)
    s1 <- s2 <- s3 <- s4 <- numeric(Tmax)
    xi1 <- rnorm(Tmax, 0, sigma)
    xi2 <- rnorm(Tmax, 0, sigma)
    xi3 <- rnorm(Tmax, 0, sigma)
    xi4 <- rnorm(Tmax, 0, sigma)
    xi5 <- rnorm(Tmax, 0, sigma)

    x1[1] <- x1o
    x2[1] <- x2o
    x3[1] <- x3o
    x4[1] <- x4o
    x5[1] <- x5o

    for (t in 1:(Tmax - 1)) {
      s1[t] <- x1[t] * (1 - u_prey)
      s2[t] <- x2[t] * (1 - u_prey)
      s3[t] <- x3[t] * (1 - u_prey)
      s4[t] <- x4[t] * (1 - u_pred)

      x1[t + 1] <- s1[t] * exp(1.0213 - s1[t] - 0.0861 * s2[t] -
        0.3141 * s3[t] - 0.7252 * s4[t] -
        0.2445 * x5[t] + xi1[t])
      x2[t + 1] <- s2[t] * exp(1.0289 - 0.4765 * s1[t] - s2[t] -
        0.1370 * s3[t] - 0.9811 * s4[t] -
        0.0915 * x5[t] + xi2[t])
      x3[t + 1] <- s3[t] * exp(1.0207 - 0.3193 * s1[t] -
        0.3461 * s2[t] - s3[t] -
        0.6367 * s4[t] - 0.8716 * x5[t] + xi3[t])
      x4[t + 1] <- s4[t] * exp(0.7252 * s1[t] + 0.9811 * s2[t] +
        0.6367 * s3[t] - s4[t] + xi4[t])
      x5[t + 1] <- x5[t] * exp(0.2445 * s1[t] + 0.0915 * s2[t] +
        0.8716 * s3[t] - x5[t] + xi5[t])
    }
    df <- dplyr::bind_rows(tibble(time = 1:Tmax, x1, x2, x3, x4, x5, r), df)
  }
  df
}
```

## Model A

```r
model_A <- function(u_prey = 0.5,
                    u_pred = 0.5,
                    sigma = 0.05,
                    x1o = 0.44, # unfished equib
                    x2o = 0.17,
                    x3o = 0.186,
                    x4o = 0.600,
                    x5o = 0.280,
                    Tmax = 50,
                    R1 = 3, # 1.15, #1.0213,
                    A11 = 8,
                    A14 = 0.9, # 0.7252,
                    A15 = 0.9, # 0.2445,
                    A41 = 0.1, # 0.7252,
                    A51 = 0.3, # 0.2445,
                    reps = 40) {
  df <- tibble()
  for (r in 1:reps) {
    x1 <- x4 <- x5 <- numeric(Tmax)
    s1 <- s4 <- numeric(Tmax)
    x2 <- x3 <- numeric(Tmax)
    xi1 <- rnorm(Tmax, 0, sigma)
    xi4 <- rnorm(Tmax, 0, sigma)
    xi5 <- rnorm(Tmax, 0, sigma)

    x1[1] <- x1o + x2o + x3o
    x4[1] <- x4o
    x5[1] <- x5o

    for (t in 1:(Tmax - 1)) {
      s1[t] <- x1[t] * (1 - u_prey)
      s4[t] <- x4[t] * (1 - u_pred)
      x1[t + 1] <- s1[t] * exp(R1 - A11 * s1[t] - A14 * s4[t] - A15 * x5[t] + xi1[t])
      x4[t + 1] <- s4[t] * exp(A41 * s1[t] - s4[t] + xi4[t])
      x5[t + 1] <- x5[t] * exp(A51 * s1[t] - x5[t] + xi5[t])
    }
    df <- bind_rows(df, tibble(time = 1:Tmax, x1, x2, x3, x4, x5, r = r))
  }
  df
}
```

## Model B

```r
model_B <- function(u_prey = 0,
                    u_predator = 0,
                    A1 = 2,
                    R1 = 0.1,
                    A2 = 2.75,
                    R2 = 1.45,
```

```
                    Tmax = 50,
                    x1o = 0.44, # unfished equib
                    x2o = 0.17,
                    x3o = 0.186,
                    x4o = 0.600,
                    x5o = 0.280,
                    sigma = 0.01,
                    reps = 40) {
  df <- tibble()
  for (r in 1:reps) {
    omega1 <- rnorm(Tmax, 0, sigma)
    omega2 <- rnorm(Tmax, 0, sigma)
    omega3 <- rnorm(Tmax, 0, sigma)

    s1 <- x1 <- numeric(Tmax)
    s4 <- x4 <- numeric(Tmax)
    x2 <- x3 <- numeric(Tmax)
    x5 <- numeric(Tmax)

    x1[1] <- x1o + x2o + x3o
    x4[1] <- x4o
    x5[1] <- x5o

    for (t in 1:(Tmax - 1)) {
      s1[t] <- x1[t] * (1 - u_prey)
      s4[t] <- x4[t] * (1 - u_predator)

      x1[t + 1] <- s1[t] * exp(R1 - s1[t] * A1 + omega1[t])
      x4[t + 1] <- s4[t] * exp(R2 - s4[t] * A2 + omega2[t])
      x5[t + 1] <- .25 * x1[t]
    }

    df <- bind_rows(df, tibble(time = 1:Tmax, x1, x2, x3, x4, x5, r = r))
  }
  df
}
```

# Optimal decision

Determine the optimal policy using Nelder-Meade simplex method provided by the `optim` function:

```
u_A <- function(x) utility(x, f = model_A)
A <- optim(c(.8, 0.02), u_A)
model_A_policy <- clip(A$par, 0, 1)
```

```
u_B <- function(x) utility(x, f = model_B)
B <- optim(c(0.01, 0.1), u_B)
model_B_policy <- clip(B$par, 0, 1)
```

```
u_true <- function(x) utility(x, f = model_5sp)
o <- optim(c(0.01, 0.5), u_true)
true_policy <- clip(o$par, 0, 1)
```

## Simulate scenarios

We simulate the system using the true model, while managing from the policy derived from forecasts of model A:

```
Tmax <- 10
reps <- 40

x <- model_A_policy
sim <- model_5sp(
  u_prey = x[[1]], u_pred = x[[2]],
  Tmax = Tmax, sigma = 0.05, reps = reps
)
obs <- sim %>%
  format_sim() %>%
  group_by(time, species) %>%
  summarize(sd = sd(biomass), biomass = mean(biomass), type = "observed")

predict <- model_A(
  u_prey = x[[1]], u_pred = x[[2]],
  Tmax = Tmax, reps = reps
) %>%
  format_sim() %>%
  group_by(time, species) %>%
  summarize(sd = sd(biomass), biomass = mean(biomass), type = "predicted")


scenario_A <- bind_rows(obs, predict) %>%
  filter(species != "herring") %>%
  mutate(scenario = "Model A")
mean_utility_A <- reward(df = sim, x = x) / reps
```

We repeat the simulation over 40 replicates using the policy derived from model B forecasts:

```
x <- model_B_policy
sim <- model_5sp(
  u_prey = x[[1]], u_pred = x[[2]],
  Tmax = Tmax, sigma = 0.05, reps = reps
)
obs <- sim %>%
  format_sim() %>%
  group_by(time, species) %>%
  summarize(sd = sd(biomass), biomass = mean(biomass), type = "observed")

predict <- model_B(
  u_prey = x[[1]], u_pred = x[[2]],
  Tmax = Tmax, reps = reps
) %>%
  format_sim() %>%
  group_by(time, species) %>%
  summarize(sd = sd(biomass), biomass = mean(biomass), type = "predicted")

scenario_B <- bind_rows(obs, predict) %>%
  filter(species != "herring") %>%
```

```
  mutate(scenario = "Model B")


mean_utility_B <- reward(df = sim, x = x) / reps
```

```
example1 <- bind_rows(scenario_A, scenario_B)
write_csv(example1, "../data/example1.csv")

example1 %>%
  ggplot(aes(time, biomass, col = species)) +
  geom_point(aes(shape = type)) +
  geom_errorbar(aes(ymin = biomass - 2 * sd, ymax = biomass + 2 * sd, lty = type)) +
  facet_wrap(~scenario)
```

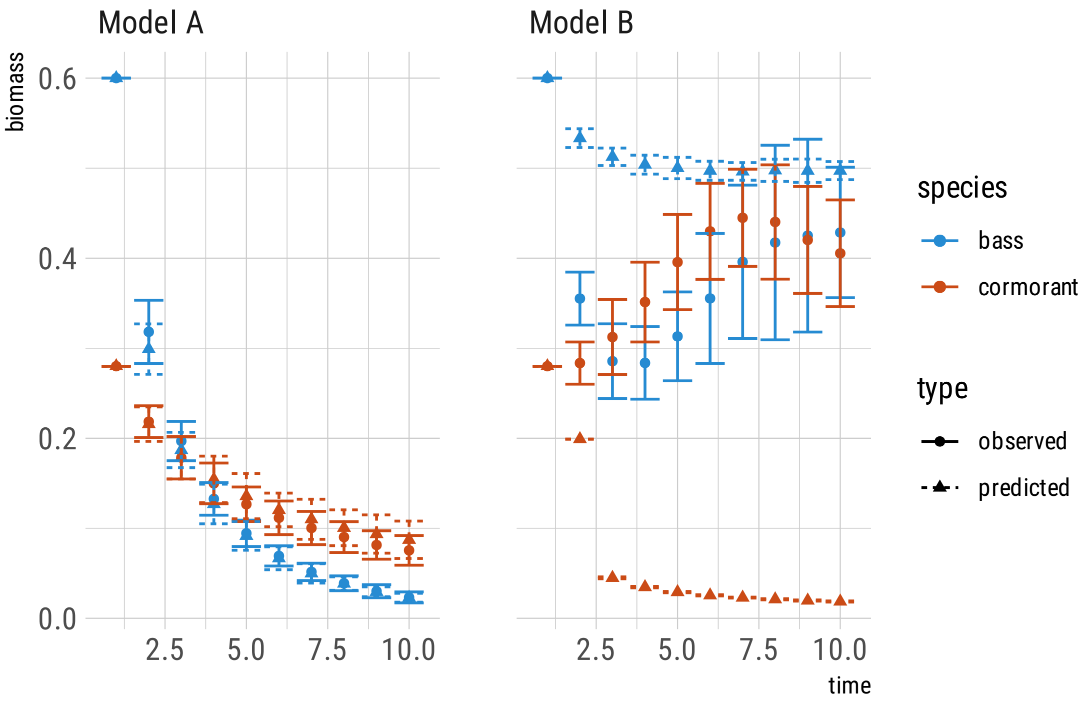


```
ratio <- mean_utility_A / mean_utility_B
```

The ratio of mean utility under model A to mean utility under the nearly-optimal model B is 41%.

# References

Brias, A. & Munch, S.B. (2021). Ecosystem based multi-species management using Empirical Dynamic Programming. *Ecological Modelling*, 441, 109423.
