# Supplementary material for: The Forecast Trap
Source: arXiv:2207.10193 source file (2022-07-20)
Supplement: Supplementary file 2 [file appendix-B.pdf]

# Appendix B: The Forecast Trap in a Sequential Decision-Making Problem

Carl Boettiger

The methods applied here – stochastic dynamic programming, iterative forecasts assessed with proper scoring rules, and adaptive management – are not themselves novel, thus the reader is referred to previous reviews and text books which can provide a thorough introduction to methods, in particular, Marescot *et al.* (2013) and Smith & Walters (1981). However, implementation of these approaches generally depends on numerical methods, for which even precise mathematical formulas or pseudo-code descriptions can be inadequate to specify unambiguously or to properly facilitate replication (Barnes 2010). As such, this appendix includes computer code in the R language, which can also be found in the corresponding R-Markdown document in the paper's GitHub repository, https://github.com/cboettig/bad-forecast-good-decision. While computer code can be more verbose and difficult to read than mathematical formulas presented here, it is also less ambiguous. Though R is already widely used among ecologists, the implementations concern mostly matrix algebra that can be translated to other languages, and the `MDPtoolbox` package used here is also implemented in MatLab (Marescot *et al.* 2013; Chades *et al.* 2017).

Below, I provide carefully annotated code necessary to completely reproduce all of the analysis presented in the main paper. This analysis is run in R (R Core Team 2020) uses `MDPtoolbox` (Chades *et al.* 2017) for solving Markov Decision Processes (MDP) using stochastic dynamic programming functionality, `expm` for matrix exponentials (Goulet *et al.* 2020), and a few custom MDP functions provided by our package, `mdplearning` (Boettiger & Memarzadeh 2020). We will also use `tidyverse` packages for basic manipulation and plotting (Wickham *et al.* 2019). This file is also available as an RMarkdown document (Xie *et al.* 2018) at https://github.com/cboettig/bad-forecast-good-decision. The code below generates the data tables required for each plot shown in the main paper. Data are stored as `.csv` tables to be accessible to any relevant software program. Plotting commands used in the main paper are embedded in the paper's RMarkdown file at https://github.com/cboettig/bad-forecast-good-decision.

## Optimal quotas as a Markov Decision Process (MDP) problem

The question of optimal harvest quotas given a population growth model can be posed as a Markov Decision Process (MDP). Marescot *et al.* (2013) provides an accessible overview of MDP problems and their solutions in conservation context. Reed (1979) provides a formal proof of optimal harvest strategy for stochastic dynamics under the assumption of any concave growth function. The problem can be summarized as follows:

A manager seeks to maximize the sum of the utility derived from such a harvest and such a state, $U(X_t, H_t)$, over all time, subject to discount rate $\delta$:

$$\sum_{t=0}^{t=\infty} U(X_t, H_t)\delta^t \tag{1}$$

While in principle the utility could reflect many things, including the cost of fishing, market responses to supply and demand, the value of recreational fishing, the intrinsic value fish left in the sea (see Halpern *et al.* 2013), for simplicity we will assume utility is merely a linear function of the harvest quota set by the manager, i.e. a fixed price $p$ per kilogram of fish harvested: $U(X_t, H_t) = p\min(H_t, X_t)$ (noting that realized

harvest cannot exceed the available stock). As units are already specified in dimensionless quantities in this example, so without loss of generality we will set $p = 1$.

To solve this optimization, we must also know the dynamics of $X_t$, describing how future stock $X_{t+1}$ changes from the present state, $X_t$, after to harvest $H_t$:

$$X_{t+1} = f(X_t, H_t) \tag{2}$$

This problem is already well studied in 1 dimension (i.e. a single species without age structure): Clark (1973) solves the optimization when $f$ is a deterministic function $f$ and Reed (1979) extended that result to the stochastic case. It is worth noting that even under the simple utility function which assigns no value to fish that are not harvested, the optimal strategy still seeks to sustain the fish population indefinitely. As Reed (1979) proves, the optimal strategy can be characterized by a policy of "constant escapement," in which the manager adjusts the harvest effort each year in an effort to ensure the same number or biomass of fish are left in the sea each year. The optimization problem can then be solved by dynamic programming, using the recursive Bellman equation. This technique, known as stochastic dynamic programming (SDP) is widely used in conservation decision problems Marescot *et al.* (2013).

It is worth noting that while constant escapement is used in the management of several important fish stocks such as salmon, most marine fisheries are not managed using this optimal solution for a fluctuating population, but instead rely on a 'constant harvest effort' (or constant "yield") policy. In the case of a deterministic model at equilibrium, these policies are identical. Though constant-effort policies are technically sub-optimal for the problem as stated above with stochastic growth, in practice they can be more robust, such as when measurements of the current stock size $X_t$ are uncertain. These issues are discussed in detail in Memarzadeh & Boettiger (2019). For our purposes, it suffices to note that constant escapement policy is relevant both from a theoretical standpoint as the optimal solution for the problem under consideration, and an applied standpoint as a policy that guides management of many salmon fisheries. The optimal control approach using SDP as illustrated here is used in a wide and growing number of conservation problems.

Bear in mind that in the example presented here, SDP merely serves the role of a convenient and established way for a manager to determine the optimal action, given some model estimation. Whether we use SDP or some other way to determine the optimal policy, given the model, is immaterial to the conclusion.

# Solving MDP via SDP

To solve the decision problem using SDP, we define the state space and the action space on a discrete grid of 240 points. The maximum state is set well above the largest carrying capacity used in the models, which limits the influence of boundary effects introduced by the transformation to a discrete, finite grid. Available harvest actions match the state space, effectively allowing any harvest level to be possible.

The utility (reward) of an action is set to the (realized) harvest (e.g. a fixed price per unit fish, with no cost applied to harvest effort), ensuring no harvest can exceed the available stock.

$$U(x_t, h_t) = p \min(x_t, h_t)$$

Future utility is discounted by fixed factor of $\delta = 0.99$. Classic maximum sustainable yield models (Schaefer 1954) ignore discounting, while modern economic optimization models insist on it, so a small discount conforms to the latter while reasonably approximating the former. The qualitative conclusion is not sensitive to the discounting rate.

Alternate reward functions with varying price and cost structures are possible but do not qualitatively impact the conclusions. This reward function is a limiting case of any more complex reward, and corresponds both to classic work that does not model utility explicitly (e.g. MSY theory, Schaefer 1954), as well as explicit assumptions typically made in more recent models (Reed 1979). Moreover, using a simple reward function makes it clear that model that performs best is not doing so merely because of particular features baked into the a carefully chosen reward rule.

## Ecological Model Definitions

Let us assume that our set of candidate models are simply the possible parameterizations of a stochastic version of the classic Gordon-Schaefer model (Gordon & Press 1954; Schaefer 1954):

$$X_{t+1} = f_i(Y_t) = Y_t + r_i Y_t \left(1 - \frac{Y_t}{K_i}\right) * \xi_t(\sigma) \tag{3}$$

where harvest occurs before recruitment, $Y_t = \min(X_t - H_t, 0)$, $\xi_i(t)$ is a multiplicative log-normal noise term with mean 1 and log-standard-deviation $\sigma_i$.

Before this or any other model can generate a forecast, we must first come up with some parameter estimates. Because the model includes (log-normal) stochastic growth, no amount of data will make any parameter combination impossible, though certain parameter values are more likely than others. Remember too that parameter estimates may be derived in other ways than than model fitting, especially when parameters are amenable to biological interpretation. We will consider the whole range of possible parameters in a moment, but for simplicity, let us begin by focusing in around two of the most interesting regions of that are already included within that larger parameter space of all possible values for $r$, $K$, and $\sigma$. Let us take "Model 1" as being given by $r_1 = 2$, $K_1 = 16$, $\sigma_1 = 0.05$, "Model 2" by $r_2 = 0.5$, $K_2 = 10$, $\sigma_2 = 0.075$. We can imagine our comparison of these two models as a microcosm of the larger comparison between all possible paremeterizations.

Ecologists will rightly scoff at the simplicity of these models – the real world is much more complicated. So it is important to bear in mind that these are not models that seek to approximate the stock dynamics of real world fisheries, only to approximate whatever "true model" we are using to drive the simulation. In recognition of the fact that real world is always more complex than even our best ecological models, we will assume a "true model" for the simulations that is not in the Gordon-Schaefer class (i.e. our candidate models will never contain the true model), but is not so rich that a Gordon-Schaefer curve would seem a hopelessly poor approximation.

For illustrative purposes, we will thus assume the "true" process to be given by Model 3, which is unknown to the decision-maker, but similar enough to at least one of the candidate models might be considered a reasonable approximation:

$$f_3(Y) = Y + r_3 Y^4 \left(1 - \frac{Y}{K_3}\right) \tag{4}$$

with $r_3 = 0.002$, $K_3 = 10$ and $\sigma_3 = 0.05$.

Certainly, the challenge of choosing which model to base a decision policy on in the real world is much harder than this binary choice between two models, and yet it is sufficient to illustrate the trap. We will see later why making the models much more complex does not guarantee that the task becomes easier or that the trap may be ruled out.

# Methods for Managing Under Model Uncertainty

I will use this example to illustrate two alternative approaches for iterative learning over model uncertainty: iterative forecasting and adaptive management. The central difference in the approaches is that iterative forecasting is premised on the ability to score the predictions of alternative models. Iterative forecasting is silent on the issue of what to do with those scores, this is left up to the decision-maker. Adaptive management approaches, by contrast, explicitly seek to integrate probabilities over all candidate models to reach a decision. I consider each in turn.

## Statistical approaches: Forecasting under "Proper" Scoring Rules

Like many decision problems, the task of setting a sustainable harvest quota appears to hinge on having an accurate forecast: if we can predict to what size the fish stock will increase next year, $X_{t+1}$, and we know the current stock, $X_t$, then we can sustainably harvest $X_{t+1} - X_t$ without decreasing the biomass over the long term. Selecting a model based on forecast skill is also justifiable on theoretical grounds, since it reduces the risk of overfitting by comparing model predictions to later observations that were not used to estimate the model (Gneiting & Katzfuss 2014).

I illustrate the process of model selection by strictly proper scoring rules using two scenarios. In Scenario A (passive observation) the fish stock is unharvested and allowed to recover towards carrying capacity (as simulated under our "true" model, Model 3) while comparing the observed stock size in each subsequent time step to the distribution predicted under model 1 and model 2 respectively [Fig 1]. The mean, $\mu_t$ and variance, $\sigma_t$ of the forecast are compared against the true observation $x_t$ using the log-likelihood proper scoring rule given by Gneiting & Raftery (2007),

$$S(x_t|\mu_t, \sigma_t) = -(\mu_t - x_t)^2/\sigma_t^2 - \log(\sigma_t) \tag{5}$$

for each prediction over 100 replicate simulations of 100 time steps each [Fig 2].

# Analysis

```r
library(tidyverse)
library(MDPtoolbox)
library(expm)
# remotes::install_github("boettiger-lab/mdplearning")
library(mdplearning)
```

```r
states <- seq(0, 24, length.out = 240)
actions <- states
obs <- states
reward_fn <- function(x, h) pmin(x, h)
discount <- 0.99

# K is at twice max of f3; 8 * K_3 / 5
f1 <- function(x, h = 0, r = 2, K = 10 * 8 / 5) {
  s <- pmax(x - h, 0)
  s + s * (r * (1 - s / K))
}
f2 <- function(x, h = 0, r = 0.5, K = 10) {
  s <- pmax(x - h, 0)
  s + s * (r * (1 - s / K))
}

# max is at 4 * K / 5
f3 <- function(x, h = 0, r = .002, K = 10) {
  s <- pmax(x - h, 0)
  s + s^4 * r * (1 - s / K)
}

## gather models together, indicate true model
```

```r
sigma_g <- 0.05
models <- list("1" = f1, "2" = f2, "3" = f3)
model_sigmas <- c(sigma_g, 1.5 * sigma_g, sigma_g)
true_model <- "3"
```

On a discrete grid of possible states and actions, we can define the growth rate of a given state $X_t$ subject to harvest $H_t$, $f(X_t, H_t)$ as set of matrices. Each matrix $i$ gives the transition probabilities for any current state to any future state, given that action $i$ is taken.

```r
transition_matrices <- function(f, states, actions, sigma_g) {
  n_s <- length(states)
  n_a <- length(actions)
  transition <- array(0, dim = c(n_s, n_s, n_a))
  for (k in 1:n_s) {
    for (i in 1:n_a) {
      nextpop <- f(states[k], actions[i])
      if (nextpop <= 0) {
        transition[k, , i] <- c(1, rep(0, n_s - 1))
      } else if (sigma_g > 0) {
        x <- dlnorm(states, log(nextpop), sdlog = sigma_g)
        if (sum(x) == 0) { ## nextpop is computationally zero
          transition[k, , i] <- c(1, rep(0, n_s - 1))
        } else {
          x <- x / sum(x) # normalize evenly
          transition[k, , i] <- x
        }
      }
    }
  }
  transition
}
```

This follows the standard setup for standard stochastic dynamic programming, see Marescot *et al.* (2013). Having defined a function to compute the transition matrix, we can use it to create matrices corresponding to each of the three models:

```r
P <- lapply(seq_along(models), function(i) {
  transition_matrices(models[[i]], states, actions, model_sigmas[[i]])
})
names(P) <- c("1", "2", "3")
```

Likewise, a corresponding matrix defining the rewards associated with each state $X$ and each harvest action $H$ can also be defined.

```r
## Compute reward matrix (shared across all models)
n_s <- length(states)
n_a <- length(actions)
reward <- array(0, dim = c(n_s, n_a))
for (k in 1:n_s) {
  for (i in 1:n_a) {
    reward[k, i] <- reward_fn(states[k], actions[i])
  }
}
```

# Optimal control solutions

We use value iteration to solve the stochastic dynamic program (Marescot *et al.* 2013; Chades *et al.* 2017) for each model. This determines the optimal harvest policy for each possible state, given each model. Because this step is the most computationally intensive routine, we cache the results using memoization conditioned on the transition matrices (Wickham *et al.* 2017). Running this code with alternate transition matrices automatically invalidates that cache, reducing the risk of loading spurious results.

```
mdp <- memoise::memoise(mdp_value_iteration,
  cache = memoise::cache_filesystem("cache/")
)

policies <-
  map_dfr(P,
    function(P) {
      soln <- mdp(P, reward,
        discount = discount,
        epsilon = 0.01, max_iter = 2000, V0 = rep(0, dim(P)[[1]])
      )
      escapement <- states - actions[soln$policy]
      tibble(states, policy = soln$policy, escapement)
    },
    .id = "model"
  )

write_csv(policies, "../data/policies.csv")
```

# Simulations and step-ahead forecasts (Fig 3, 4A)

We simulate fishing dynamics under the optimal policy for each model, using a simple helper function from the `mdplearning` package. Because growth dynamics are stochastic, we perform 100 simulations of each model from identical starting condition to ensure results are not the result of chance alone.

```
library(mdplearning)
Tmax <- 100
x0 <- which.min(abs(states - 6))
reps <- 100
set.seed(12345)

## Simulate each policy reps times, with `3` as the true model:
simulate_policy <- function(i, policy) {
  mdp_planning(P[[true_model]], reward, discount,
    policy = policy, x0 = x0, Tmax = Tmax
  ) %>%
    select(value, state_index = state, time, action_index = action) %>%
    mutate(state = states[state_index])
}

sims <-
  map_dfr(names(P),
    function(m) {
      policy <- policies %>%
```

```
        filter(model == m) %>%
        pull(policy)
      map_dfr(1:reps, simulate_policy, policy = policy, .id = "reps")
    },
    .id = "model"
  )

write_csv(sims, "../data/sims.csv")
```

Using the transition matrices directly, we can examine what each model would have forecast the future stock size to be in the following year when no fishing occurs (note that for each model, we use the transition matrix that corresponds to 'no fishing', `model[[state_index, ,1]]`) (Fig 2A, main text). The transition matrices give the full (discretized) probability distribution, from which we can easily calculate both the expected value and the 95% confidence interval.

```
stepahead_unfished <- sims
stepahead_unfished$state_index <- rep(sims$state_index[sims$model == "1"], 3)


stepahead_unfished <- stepahead_unfished %>%
  filter(model != "3") %>%
  mutate(next_state = dplyr::lead(state_index), model = as.integer(model)) %>%
  rowwise() %>%
  mutate(
    expected = as.numeric(P[[model]][state_index, , 1] %*% states),
    var = P[[model]][state_index, , 1] %*% states^2 - expected^2,
    low = states[max(which(cumsum(P[[model]][state_index, , 1]) < 0.025))],
    high = states[min(which(cumsum(P[[model]][state_index, , 1]) > 0.975))],
    true = states[next_state]
  )
```

We also look at the forecast each model makes when implementing the corresponding optimal harvest:

```
stepahead_fished <- sims %>%
  filter(model != "3") %>%
  mutate(next_state = dplyr::lead(state_index), model = as.integer(model)) %>%
  rowwise() %>%
  mutate(
    prob = P[[model]][state_index, next_state, action_index],
    expected = as.numeric(P[[model]][state_index, , action_index] %*% states),
    var = P[[model]][state_index, , action_index] %*% states^2 - expected^2,
    low = states[max(which(cumsum(P[[model]][state_index, , action_index]) < 0.025))],
    high = states[min(which(cumsum(P[[model]][state_index, , action_index]) > 0.975))],
    true = states[next_state]
  ) %>%
  select(time, model, true, expected, low, high, var, prob, reps)
```

# Proper scores (Fig 2C-D)

It is straight forward to apply the proper scoring formula of Gneiting & Raftery (2007) based on the first two moments of the distribution to score the respective forecasts under both the un-fished and actively managed scenario for each model:

```r
# Gneiting & Raferty (2007), eq27
scoring_fn <- function(x, mu, sigma) {
  as.numeric(-(mu - x)^2 / sigma^2 - log(sigma))
}

stepahead_unfished <- stepahead_unfished %>%
  mutate(
    sd = sqrt(var),
    score = scoring_fn(expected, true, sd)
  )

stepahead_fished <- stepahead_fished %>%
  mutate(
    sd = sqrt(var),
    score = scoring_fn(expected, true, sd)
  )
```

We store the replicate predictions under each model at each timestep, along with the scores, in a `predictions.csv` table for plotting.

```r
predictions <-
  stepahead_unfished %>%
  select(time, model, reps, expected, low, high, true, score) %>%
  mutate(scenario = "A_unfished") %>%
  bind_rows(stepahead_fished %>%
    select(time, model, reps, expected, low, high, true, score) %>%
    mutate(scenario = "B_fished")) %>%
  mutate(model = as.character(model))


write_csv(predictions, "../data/predictions.csv")
```

# Economic value tabulation (Fig 3B)

To plot the economic value over time, we must sum up the discounted values at each time step, and then average over replicate simulations of each model:

```r
##  Net Present Value accumulates over time
npv_df <- sims %>%
  group_by(model, reps) %>%
  mutate(npv = cumsum(value * discount^time)) %>%
  group_by(time, model) %>%
  summarise(mean_npv = mean(npv), .groups = "drop") %>%
  arrange(model, time)

write_csv(npv_df, "../data/npv_df.csv")
```

# Adaptive Management

Passive adaptive management using a Bayesian learning scheme still learns the wrong model. Adaptive management for MDP problems is particularly computationally intensive, and not directly supported by

the `MDPtoolbox` implementation. Nevertheless, the principle involves only a relatively straightforward, if not particularly efficient extension to the task of solving and MDP problem for a single model shown above. Given a set of transition probability matrices $P_i$ and a belief probability $b_i$ that the $i$th model is correct, it simple to define the transition matrices over possible models by the laws of conditional probability, $P = \sum_i P_i b_i$, given $\sum_i b_i = 1$. After each subsequent action and then new observation x_j, the $b_i$ probabilities for each model are updated according to Bayes law: if $b_i = P(M_i)$ is the prior probability that the model $M_i$ is correct, then the posterior probability that model $M_i$ is correct given observation $x_j$ is:

$$b_i' = P(M_i|x_j) = P(M_i)P(x_j|M_i) = b_i P(x_j|M_i)$$

Note that because the transition matrices are now altered after every action and observation, it is necessary to repeat the complete SDP calculation to determine the optimal action given the updated uncertainty. While straight forward, this is what makes adaptive management for MDP problems particularly computationally intensive and thus poorly suited for handling a large space of candidate models. Nevertheless, our example of two models is most feasible, and even the larger example of 36 models is not unreasonable. Here I make use of the `mdplearning` R package, which provides a straight-forward implementation of this algorithm.

```
adaptive_management <- memoise::memoise(mdp_learning, cache = memoise::cache_filesystem("cache/"))
am1 <- adaptive_management(P[1:2], reward, discount,
  model_prior = c(0.99, 0.01), x0 = x0,
  Tmax = 50, true_transition = P[[3]],
  epsilon = 0.001, max_iter = 2000
)
```

I also compare the adaptive management solution to an approach which still integrates uncertainty over both models, but treats the resulting policy as fixed for the duration of management, rather than adaptive *learning* by updating probabilities. This approach is sometimes referred to as uncertainty "planning," as it accounts for the same initial uncertainty over models but does not attempt to learn. For consistency, I use the same model prior as in the learning case, which heavily favors model 1 to begin with. Not surprisingly, the resulting policy is nearly identical to that under model 1 alone.

```
# Compute policy using SDP over both models, given fixed prior beliefs
policy_planning <- memoise::memoise(mdp_compute_policy, cache = memoise::cache_filesystem("cache/"))
policy <- policy_planning(P[1:2],
  reward = reward,
  discount = discount,
  model_prior = c(0.99, 0.01),
  Tmax = 50,
  epsilon = 0.001,
  max_iter = 2000
)
```

```
# Simulate under true model using fixed planning policy
non_am <- mdp_planning(P[[3]],
  reward = reward,
  discount = discount,
  model_prior = c(0.99, 0.01),
  x0 = x0,
  a0 = 1,
  policy = policy$policy,
  Tmax = 50
) %>%
  mutate(
```

```
    belief = 0.99, # belief in model 1 is fixed
    method = "planning"
  )
```

We combine results of the two methods and store the resulting `data.frame` of stock size, quota, and belief in Model 1 over time as `am.csv` for later plotting.

```
am <- am1$df %>%
  mutate(
    belief = am1$posterior$V1,
    method = "learning"
  ) %>%
  bind_rows(non_am) %>%
  mutate(
    stock = states[state],
    quota = actions[action]
  ) %>%
  select(time, stock, quota, belief, method)

write_csv(am, "../data/am.csv")
```

We can also compare these results to the net economic value achieved under Model 1 alone:

```
# tabular comparisons
npv <- npv_df %>%
  group_by(model) %>%
  summarize(npv = max(mean_npv))

am_npv <- am %>%
  group_by(method) %>%
  summarize(npv = sum(quota * discount^time))
learning <- am_npv %>%
  filter(method == "learning") %>%
  pull(npv)
am_economics_percent <- round(learning / npv[[1, "npv"]] * 100)

mean_state <- sims %>%
  group_by(model) %>%
  summarize(state = mean(state)) %>%
  filter(model == 1) %>%
  pull(state)
learn_state <- am %>%
  group_by(method) %>%
  summarize(state = mean(stock)) %>%
  filter(method == "learning") %>%
  pull(state)


am_ecology_percent <- round(learn_state / mean_state * 100)
```

Under adaptive management, the manager realizes only 38% of the economic value that would be achieved under Model 1 alone, and only 59% of the spawning stock biomass that would have been achieved under Model 1 alone.

## Adaptive management over many models

We repeat the analysis above over a grid of $r$ and $K$ values.

```
# compare over grid set of candidate r and K
rs <- c(0.01, 0.1, 0.2, 0.3, 0.4, 0.5, 2)
Ks <- c(0.5, 1, 1.5, 4, 10, 16)
sigma <- 0.1
n_models <- length(rs) * length(Ks)
pars <- expand.grid(rs, Ks)
names(pars) <- c("r", "K")
pars$sigma <- 0.1
closure <- function(r, K) {
  function(x, h = 0) {
    s <- pmax(x - h, 0)
    s + s * (r * (1 - s / K))
  }
}
many_models <- lapply(1:n_models, function(i) closure(pars[i, "r"], pars[i, "K"]))

# transition matrices
many_transitions <- lapply(seq_along(many_models), function(i) {
  transition_matrices(many_models[[i]], states, actions, sigma)
})
names(many_transitions) <- as.character(seq_along(many_models))
true_transition <- transition_matrices(f3, states, actions, sigma_g)

## Once again, initial belief favors "model 1"
model_prior <- c(rep(.01, n_models - 1) / (n_models - 1), .99)
```

With the transition matrices defined for all 42 models, we perform adaptive management as before:

```
adaptive_management <- memoise::memoise(mdp_learning,
  cache = memoise::cache_filesystem("cache/")
)
am_many <- adaptive_management(many_transitions,
  reward = reward,
  discount = discount,
  model_prior = model_prior,
  x0 = x0,
  Tmax = 20,
  true_transition = true_transition,
  epsilon = 0.001,
  max_iter = 2000
)
```

As before, we can compare the adaptive learning case to the policy which accounts for the initial uncertainty over all 42 models, but does not seek to learn.

```
policy_many <- policy_planning(many_transitions,
  reward = reward, discount = discount,
  model_prior = model_prior, Tmax = 20,
  epsilon = 0.001, max_iter = 2000
```

```
)

non_am_many <- mdp_planning(true_transition,
  reward = reward,
  discount = discount,
  model_prior = model_prior,
  x0 = x0,
  a0 = 1,
  policy = policy_many$policy,
  Tmax = 20
) %>%
  mutate(
    belief = 0.99, # belief in model 1 is fixed
    method = "planning"
  )
```

Again we record the posterior belief in the 'model 1' parameter values, and stack the data frames for learning and planning-only cases into a single file used to generate figure 4B.

```
model1 <- dim(am_many$posterior)[2]
am_multi <- am_many$df %>%
  mutate(
    belief = am_many$posterior[, model1],
    method = "learning"
  ) %>%
  bind_rows(non_am_many) %>%
  mutate(
    stock = states[state],
    quota = actions[action]
  ) %>%
  select(time, belief, stock, quota, method)

write_csv(am_multi, "../data/am_multi.csv")
```

## Posteriors

With 42 possible models instead of two, the probability weight (belief) in Model 1 does not fully capture the evolution of the belief probabilities over time. To better illustrate how these beliefs evolve over the course of the simulation, I plot the marginal probabilities over values of $r$ and $K$ across the models over time. Note that Model 1 values, $r = 2$, $K = 16$, are quickly disfavored.

```
posteriors <-
  data.frame(model = as.character(1:n_models), t(am_many$posterior)) %>%
  left_join(mutate(pars, model = as.character(1:n_models))) %>%
  pivot_longer(starts_with("X"),
    values_to = "probability",
    names_to = "time"
  ) %>%
  mutate(time = as.integer(as.factor(time)))

r_marginals <- posteriors %>%
  group_by(time, r) %>%
```

```
  summarise(prob = sum(probability), .groups = "drop")

K_marginals <- posteriors %>%
  group_by(time, K) %>%
  summarise(prob = sum(probability), .groups = "drop")
```

From the table of marginal probabilities, we generate the corresponding plots

```
belief_r <- r_marginals %>%
  mutate(r = as.character(r)) %>%
  ggplot(aes(time, prob, group = r, col = r)) +
  geom_line() +
  geom_point()


belief_K <- K_marginals %>%
  mutate(K = as.character(K)) %>%
  ggplot(aes(time, prob, group = K, col = K)) +
  geom_line() +
  geom_point()

belief_r + belief_K
```

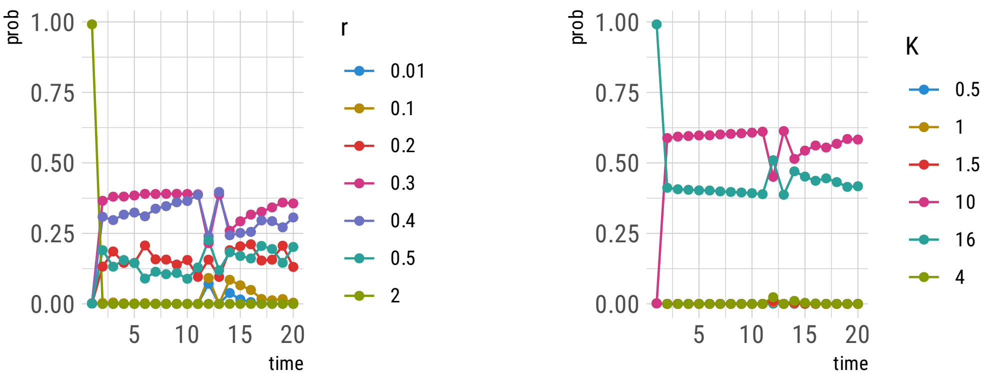


Figure 1: Fig S1: Marginal probabilities of parameters $r$ and $K$ over the course of adaptive management over all 42 models.

For most of the simulation, the most probable $r$ value is around 0.3, and the most probable $K$ value around 10.

# Growth models

To plot growth curves of individual models (Fig 5A), we evaluate

$$\Delta x = x_{t+1} - x_t = f(x_t) - x_t$$

for each model for all possible states $x_t$.

```
model_curves <-
  map_dfc(models, function(f) f(states) - states) %>%
  mutate(state = states) %>%
  pivot_longer(names(models), "model")

write_csv(model_curves, "../data/model_curves.csv")
```

The resulting model curves are shown in the main paper, Fig 5A.

# Growth models in the many-models case

The corresponding figure for the case of 42 models.

```
final_belief <- posteriors %>%
  filter(time == max(time)) %>%
  select(model, belief = probability) %>%
  mutate(type = "candidate") %>%
  bind_rows(data.frame(belief = 1, model = "true", type = "true"))

model_set <- c(f3, many_models)
names(model_set) <- c("true", 1:length(many_models))
d <-
  map_dfc(model_set, function(f) f(states) - states) %>%
  mutate(state = states) %>%
  pivot_longer(names(model_set), "model") %>%
  left_join(final_belief)

d %>%
  ggplot(aes(state, value, group = model, col = type, alpha = belief)) +
  geom_line(lwd = 1) +
  coord_cartesian(ylim = c(-5, 8), xlim = c(0, 16)) +
  ylab(bquote(f(x) - x)) +
  xlab("x")
```

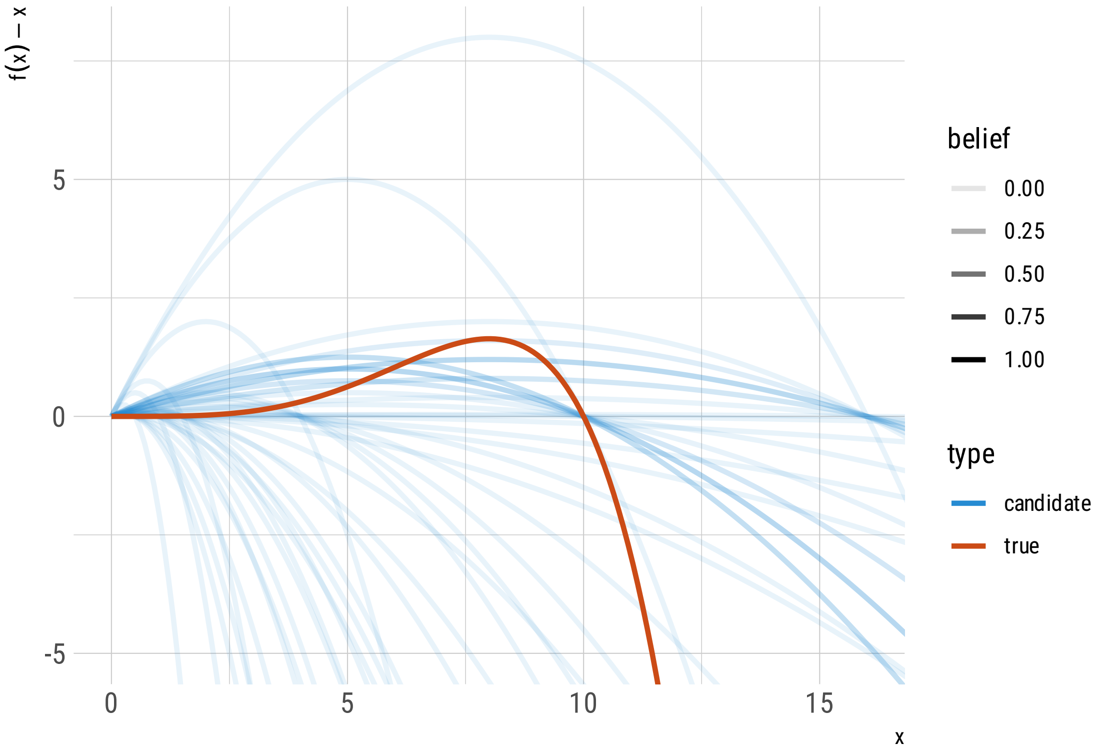


Figure 2: growth curves for 42 candidate models, shaded by belief at timestep 20, relative to the true model. The curve with parameter values corresponding to 'model 1' are recognized in the highest arc, with belief weight of less than 1%.

# References

Barnes, N. (2010). Publish your computer code: It is good enough. *Nature*, 467, 753–753.

Boettiger, C. & Memarzadeh, M. (2020). *Mdplearning: Bayesian learning algorithms for markov decision processes.*

Chades, I., Chapron, G., Cros, M.-J., Garcia, F. & Sabbadin, R. (2017). *MDPtoolbox: Markov decision processes toolbox.*

Clark, C.W. (1973). Profit maximization and the extinction of animal species. *Journal of Political Economy*, 81, 950–961.

Gneiting, T. & Katzfuss, M. (2014). Probabilistic Forecasting. *Annual Review of Statistics and Its Application*, 1, 125–151.

Gneiting, T. & Raftery, A.E. (2007). Strictly Proper Scoring Rules, Prediction, and Estimation. *Journal of the American Statistical Association*, 102, 359–378.

Gordon, H.S. & Press, C. (1954). The Economic Theory of a Common-Property Resource: The Fishery. *Journal of Political Economy*, 62, 124–142.

Goulet, V., Dutang, C., Maechler, M., Firth, D., Shapira, M. & Stadelmann, M. (2020). *Expm: Matrix exponential, log, 'etc'.*

Halpern, B.S., Klein, C.J., Brown, C.J., Beger, M., Grantham, H.S., Mangubhai, S., *et al.* (2013). Achieving the triple bottom line in the face of inherent trade-offs among social equity, economic return, and conservation. *Proceedings of the National Academy of Sciences*, 110, 6229–34.

Mangel, M. (1985). Decision and control in uncertain resource systems, 255.

Marescot, L., Chapron, G., Chadès, I., Fackler, P.L., Duchamp, C., Marboutin, E., *et al.* (2013). Complex decisions made simple: A primer on stochastic dynamic programming. *Methods in Ecology and Evolution*, 4, 872–884.

Memarzadeh, M. & Boettiger, C. (2019). Resolving the measurement uncertainty paradox in ecological management. *The American Naturalist*, 193, 645–660.

R Core Team. (2020). *R: A language and environment for statistical computing.* R Foundation for Statistical Computing, Vienna, Austria.

Reed, W.J. (1979). Optimal escapement levels in stochastic and deterministic harvesting models. *Journal of Environmental Economics and Management*, 6, 350–363.

Schaefer, M.B. (1954). Some aspects of the dynamics of populations important to the management of the commercial marine fisheries. *Bulletin of the Inter-American Tropical Tuna Commission*, 1, 27–56.

Smith, A.D.M. & Walters, C.J. (1981). Adaptive Management of Stock–Recruitment Systems. *Canadian Journal of Fisheries and Aquatic Sciences*, 38, 690–703.

Wickham, H., Averick, M., Bryan, J., Chang, W., McGowan, L.D., François, R., *et al.* (2019). Welcome to the tidyverse. *Journal of Open Source Software*, 4, 1686.

Wickham, H., Hester, J., Müller, K. & Cook, D. (2017). *Memoise: Memoisation of functions.*

Xie, Y., Allaire, J.J. & Grolemund, G. (2018). *R markdown: The definitive guide.* Chapman; Hall/CRC, Boca Raton, Florida.
